# Supplementary material for: Large-scale Urban Facility Location Selection with Knowledge-informed Reinforcement Learning
Source: arXiv:2409.01588 source file (2024-09-06)
Supplement: Supplementary file 1 [file appendix.tex]

% \clearpage
% \newpage
\appendix
\section*{Appendix}
% \section{UI of the Deployed Geospatial Application}
\begin{figure*}[t]
    \centering
    \includegraphics[width=0.99\linewidth]{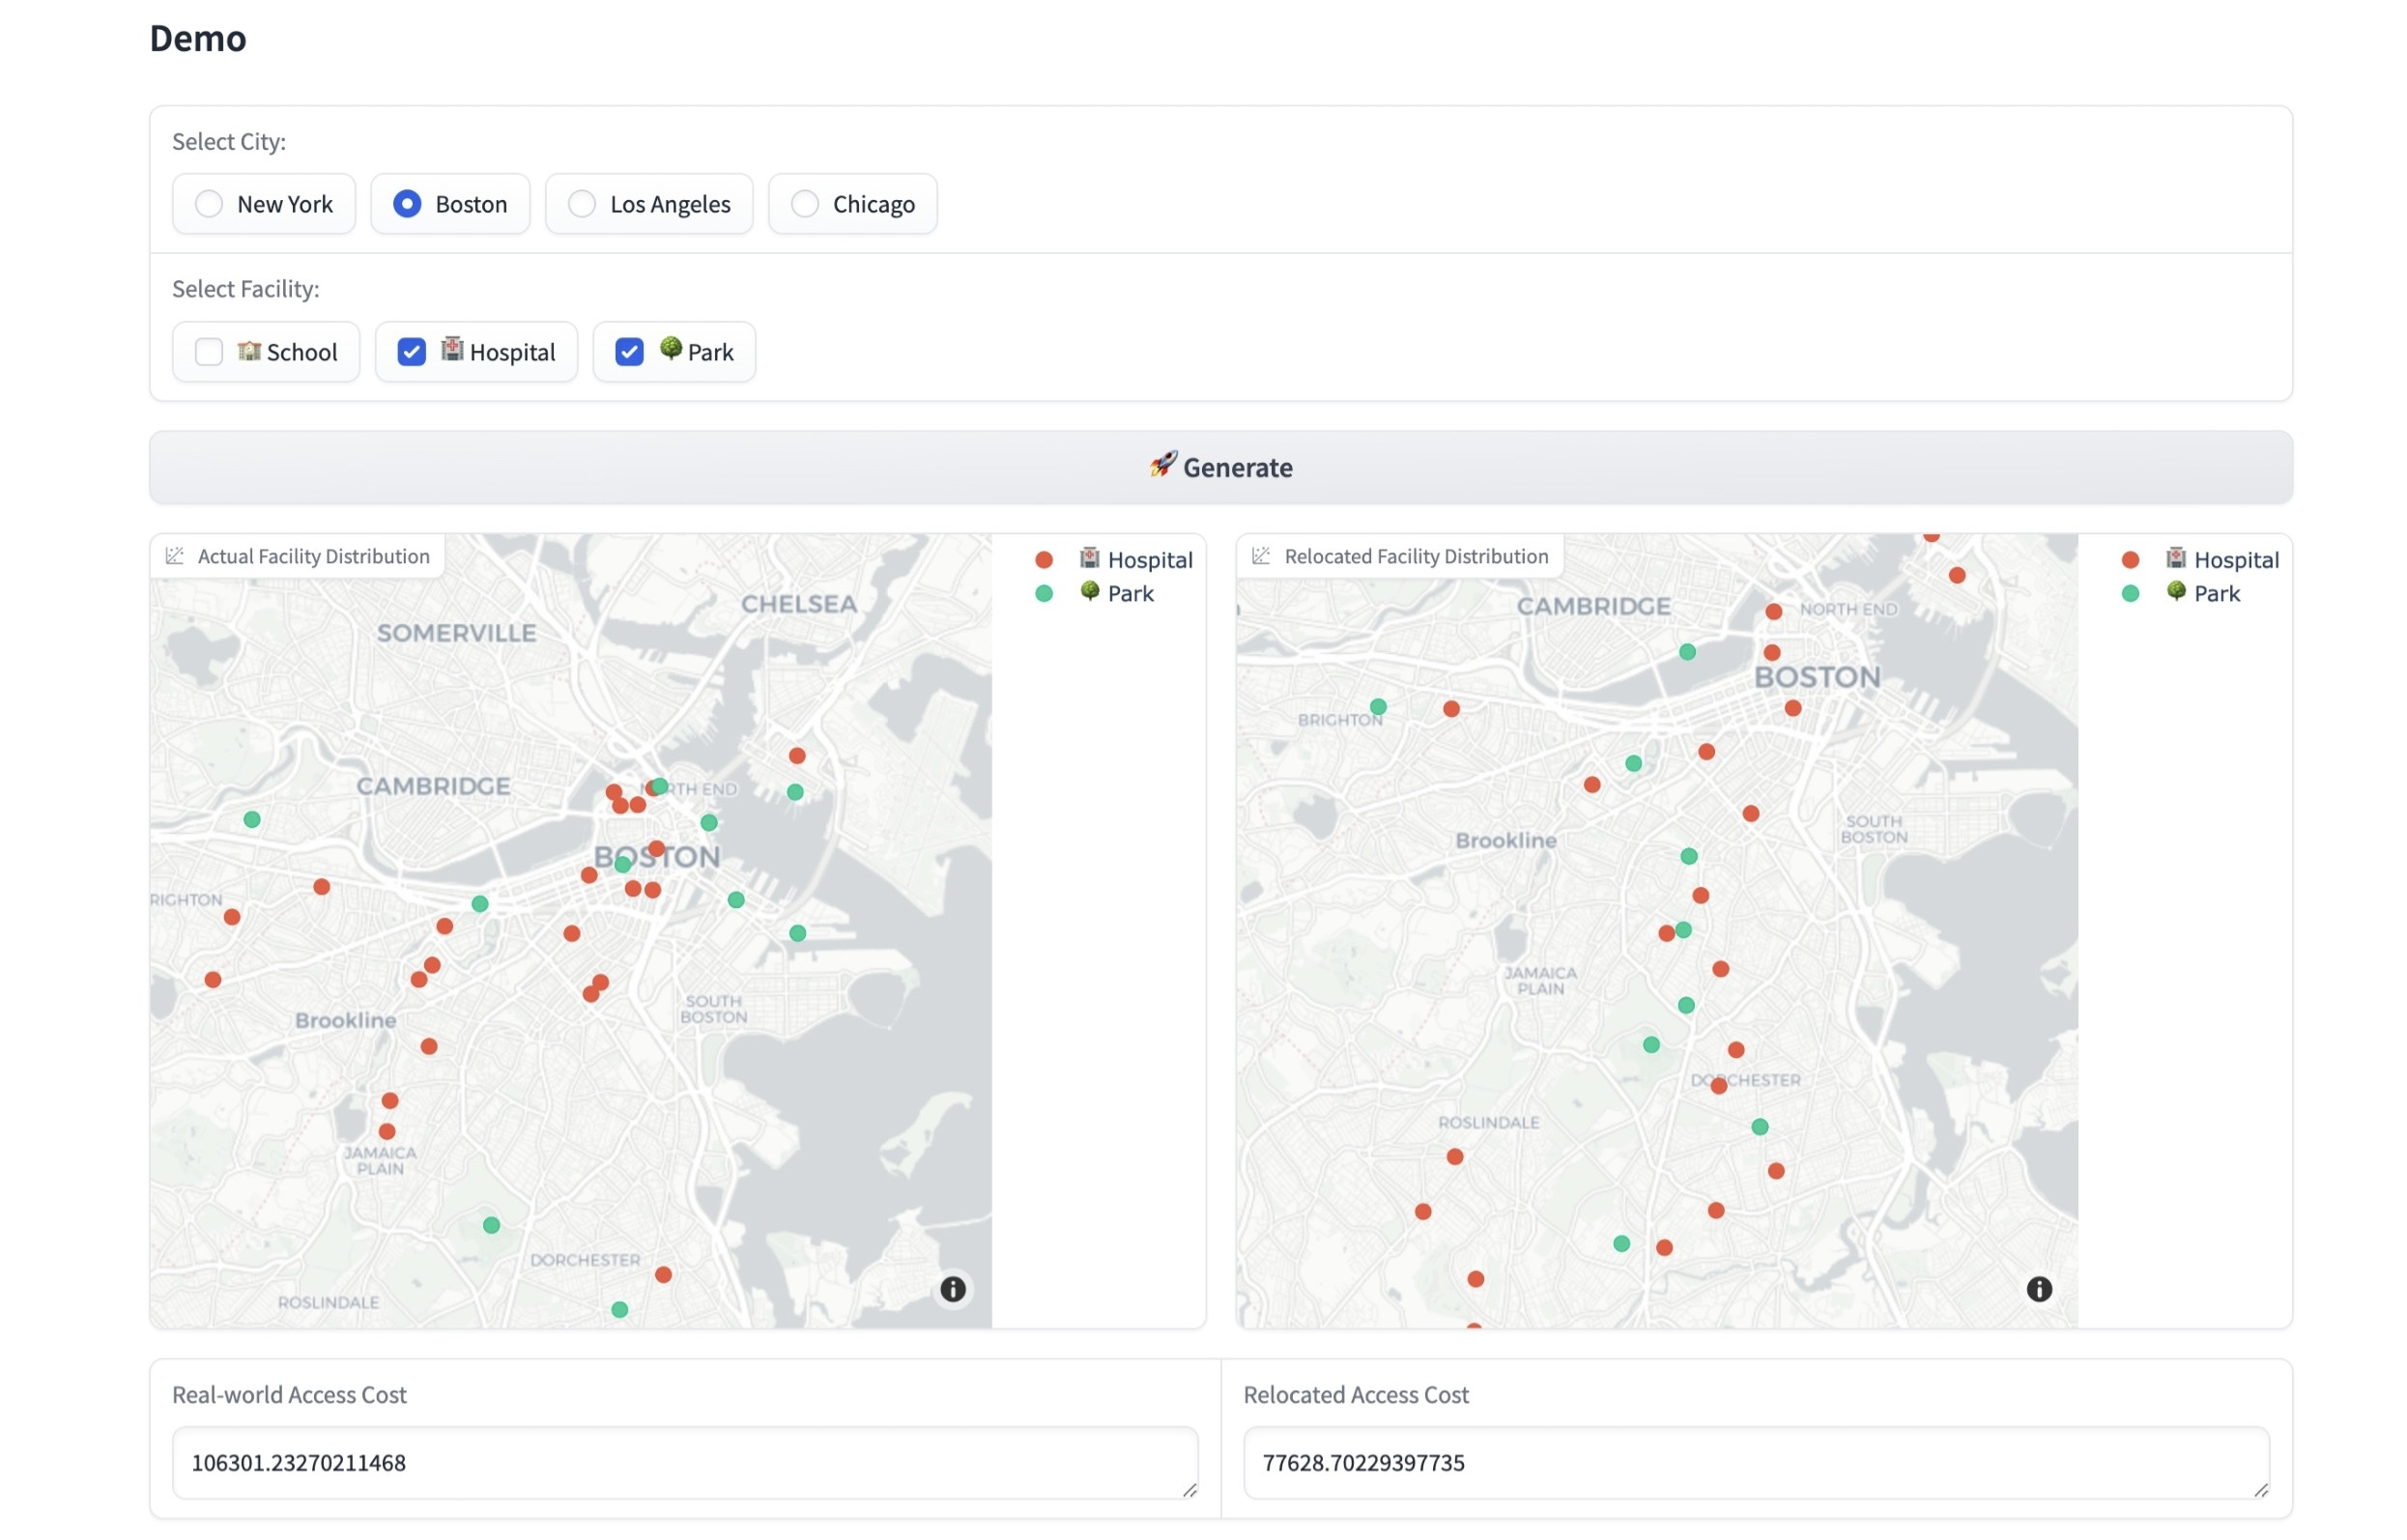}
    % \vspace{-12px}
    \caption{User interface of facility relocation for four US cities.}
    \label{fig:UI-1}
    % \vspace{-1px}
\end{figure*}

\begin{figure*}[t]
    \centering
    \includegraphics[width=0.99\linewidth]{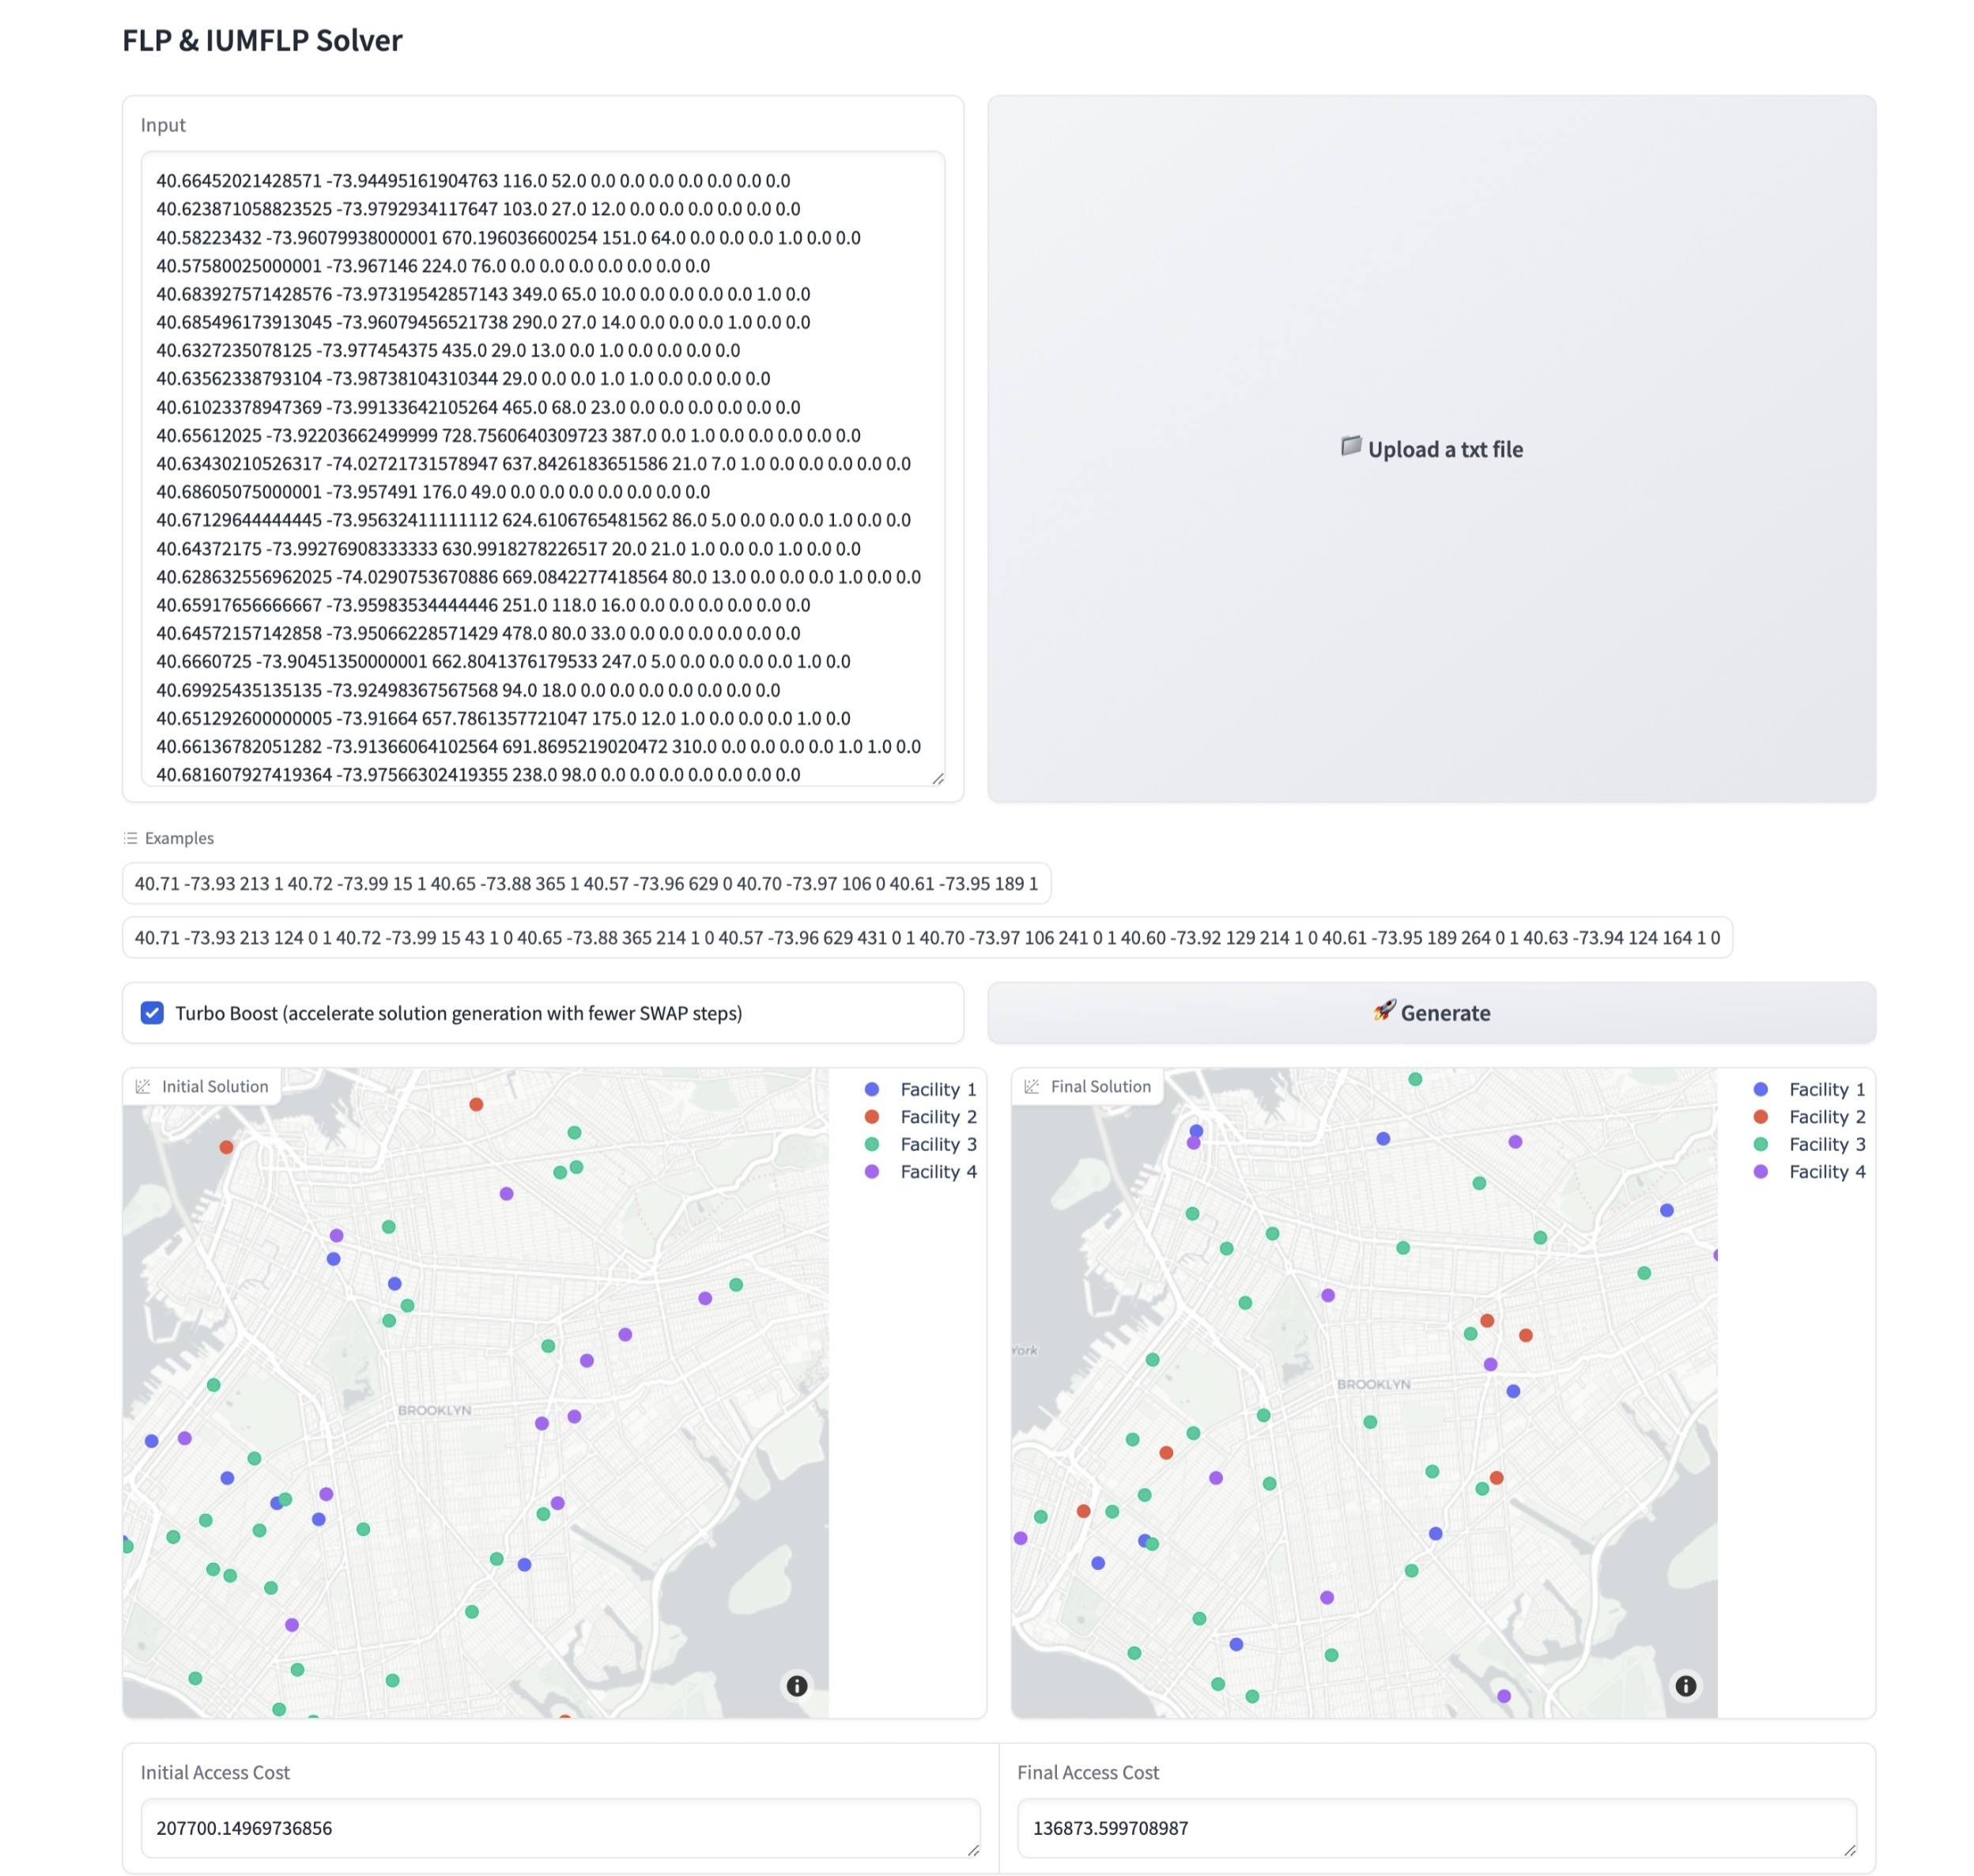}
    % \vspace{-12px}
    \caption{User interface of FLP and IUMFLP solver.}
    \label{fig:UI-2}
    % \vspace{-1px}
\end{figure*}
